# Supplementary material for: TARZAN: A Region-Based Library for Forward and Backward Reachability of Timed Automata (Extended Version)
Source: arXiv:2602.15435 source file (2026-02-17)
Supplement: Supplementary file 1 [file boolean.tex]

\begin{figure}[tb]
\begin{center}
\begin{tikzpicture}[
    ->,
    >=stealth',
    shorten >=2pt, 
    auto,
    transform shape,
    align=center,
    state/.style={thick, circle, draw, minimum size=1cm}
] 
%\useasboundingbox (-2, -3.1) rectangle (2.9, 1.71);

  \node[state, accepting] (q) {$q_0$};
  \node[state, right=2cm of q] (q1) {$q_1$};
  
  \draw [thick] 
  % Edges and loops
  (q) edge[in=150, out=30]  
  node[xshift=0pt, yshift=0pt]  
  {$x_i = i$ \\ $\mathbf{x}_{\boldsymbol{i}} \boldsymbol{:=} \mathbf{0}, \boldsymbol{ctr_i} \boldsymbol{:=} \mathbf{1} \mathbf{-} \boldsymbol{ctr_i}$} (q1)

  (q1) edge[in=330, out=210]  
  node[xshift=0pt, yshift=0pt]  
  {$x_i = i$ \\ $\mathbf{x}_{\boldsymbol{i}} \boldsymbol{:=} \mathbf{0}, \boldsymbol{ctr_i} \boldsymbol{:=} \mathbf{1} \mathbf{-} \boldsymbol{ctr_i}$} (q);

  %\draw[red, thick, dashed] (current bounding box.south west) rectangle (current bounding box.north east);
\end{tikzpicture}
\end{center}
\caption{boolean}
\label{fig:boolean}
\end{figure}
