# Supplementary material for: TARZAN: A Region-Based Library for Forward and Backward Reachability of Timed Automata (Extended Version)
Source: arXiv:2602.15435 source file (2026-02-17)
Supplement: Supplementary file 2 [file flower.tex]

\begin{figure}[tb]
\begin{center}
\begin{tikzpicture}[
    ->,
    >=stealth',
    shorten >=2pt, 
    auto,
    transform shape,
    align=center,
    state/.style={thick, circle, draw, minimum size=1cm}
] 
\useasboundingbox (-2, -3.1) rectangle (2.9, 1.71);

  % Main state
  \node[state, accepting] (q) {$q_0$};
  % Goal state below
  \node[state, below of=q, yshift=-1.5cm] (goal) {$\mathit{Goal}$};
  % Ellipsis to suggest more loops (slightly above q)
  \node[above=1cm of q, xshift=23pt, yshift=-37pt] (dots) {\Large $\mathbf{\cdots}$};
  \draw [thick] 
  % Edges and loops
  (q) edge[loop, in=180, out=240, looseness=8]  node[below, xshift=0pt, yshift=-6pt]  {$x_1 = 1$ \\ $\resetClock{x_1}$} (q)
  
  (q) edge[loop, in=90, out=150, looseness=8] node[right, xshift=21pt, yshift=0pt] {$x_2 = 2$ \\ $\resetClock{x_2}$} (q)
  
  (q) edge[loop, in=300, out=0, looseness=8] node[right, xshift=1pt, yshift=5pt] {$x_n = n$ \\ $\resetClock{x_n}$} (q)
  
  (q) edge node[right, yshift=-13pt] {$x_1 = \cdots = x_n = 0$ \\ $\land \; y \geq 1$} (goal);

  %\draw[red, thick, dashed] (current bounding box.south west) rectangle (current bounding box.north east);
\end{tikzpicture}
\end{center}
\caption{flower}
\label{fig:flower}
\end{figure}
