# Supplementary material for: TARZAN: A Region-Based Library for Forward and Backward Reachability of Timed Automata (Extended Version)
Source: arXiv:2602.15435 source file (2026-02-17)
Supplement: Supplementary file 3 [file gates.tex]

\begin{figure}[tb]
\begin{center}
\begin{tikzpicture}[
    ->,
    >=stealth',
    shorten >=2pt, 
    auto,
    transform shape,
    align=center,
    state/.style={thick, circle, draw, minimum size=1cm}
] 
 
  % First row
  \node[state, accepting] (q) {$q_0$};
  \node[state, right=2cm of q] (q1) {$q_1$};
  \node[state, right=2cm of q1] (q2) {$q_{i-1}$};
  \node[state, right=2cm of q2] (q3) {$q_i$};
  
  % Edges for first row
  \draw[thick, ->] (q) --  node[below] {$x_i = i$ \\ $\mathbf{x}_{\boldsymbol{i}} \boldsymbol{:=} \mathbf{0}$} (q1);
  \draw[thick, -] (q1) -- ($(q1)!0.3!(q2)$);
  \draw[thick, dashed, -] ($(q1)!0.3!(q2)$) -- ($(q1)!0.65!(q2)$);
  \draw[thick, ->] ($(q1)!0.65!(q2)$) -- (q2);
  \draw[thick, ->] (q2) --  node[below] {$x_i = i$ \\ $\boldsymbol{gate} \boldsymbol{:=} \boldsymbol{gate} \mathbf{+} \mathbf{1}$} (q3);
  
  % Second row (below first)
  \node[state, accepting, below=0.6cm of q] (p) {$q_0$};
  \node[state, right=2cm of p] (p1) {$q_1$};
  \node[state, right=2cm of p1] (p2) {$q_{K - 1}$};
  \node[state, right=2cm of p2] (p3) {$q_K$};
  
  % Edges for second row
  \draw[thick, ->] (p) --  node[below] {$x = K - 1$ \\ $\resetClock{x}$} (p1);
  \draw[thick, -] (p1) -- ($(p1)!0.3!(p2)$);
  \draw[thick, dashed, -] ($(p1)!0.3!(p2)$) -- ($(p1)!0.65!(p2)$);
  \draw[thick, ->] ($(p1)!0.65!(p2)$) -- (p2);
  \draw[thick, ->] (p2) --  node[below] {$x = K - 1$ \\ $\land \; \mathit{gate} = K - 1$} (p3);

   %\draw[red, thick, dashed] (current bounding box.south west) rectangle (current bounding box.north east);
   
\end{tikzpicture}
\end{center}
\caption{gates}
\label{fig:gates}
\end{figure}
