# Supplementary material for: TARZAN: A Region-Based Library for Forward and Backward Reachability of Timed Automata (Extended Version)
Source: arXiv:2602.15435 source file (2026-02-17)
Supplement: Supplementary file 4 [file ring.tex]

\begin{figure}[tb]
\begin{center}
\begin{tikzpicture}[
    ->,
    >=stealth',
    shorten >=2pt, 
    auto,
    transform shape,
    align=center,
    state/.style={thick, circle, draw, minimum size=1cm}
] 
 
  % First row
  \node[state, accepting] (q) {$q_0$};
  \node[state, right=2cm of q] (q1) {$q_1$};
  \node[state, below=1.2cm of q1] (q2) {$q_4$};
  \node[state, left=2cm of q2] (q3) {$q_5$};
  
  % Edges for first row
  \draw[thick, ->] (q) --  node[above] {$x_i = i$ \\ $\mathbf{x}_{\boldsymbol{i}} \boldsymbol{:=} \mathbf{0}$} (q1);
  \draw[thick, -] (q1) -- ($(q1)!0.35!(q2)$);
  \draw[thick, dashed, -] ($(q1)!0.35!(q2)$) -- ($(q1)!0.53!(q2)$);
  \draw[thick, ->] ($(q1)!0.53!(q2)$) -- (q2);
  \draw[thick, ->] (q2) --  node[below] {$x_i = i$ \\ $\mathbf{x}_{\boldsymbol{i}} \boldsymbol{:=} \mathbf{0}$} (q3);
  \draw[thick, ->] (q3) --  node[right] {$x_i = i$ \\ $\mathbf{x}_{\boldsymbol{i}} \boldsymbol{:=} \mathbf{0}$} (q);

   %\draw[red, thick, dashed] (current bounding box.south west) rectangle (current bounding box.north east);
   
\end{tikzpicture}
\end{center}
\caption{ring}
\label{fig:ring}
\end{figure}
