# Supplementary material for: TARZAN: A Region-Based Library for Forward and Backward Reachability of Timed Automata (Extended Version)
Source: arXiv:2602.15435 source file (2026-02-17)
Supplement: Supplementary file 5 [file auxiliary_algorithms.tex]

\begin{algorithm}[t]
    \caption{\texttt{insert-right}$(\reg, \algx, i)$}
    \label{alg:finddelaysucc}
    
    \KwData{$\reg$: a region;
    $\algx$: the new set of clocks to insert in $\reg$;
    $i$: an index specifying the position in $\reg$ to the right of which $\algx$ is inserted;}
    \KwResult{\emph{None}, as the changes are applied directly to $\reg$.}
    \Begin() {
         \If{$(i < -q_{\reg}) \lor (i > p_{\reg})$}{
             \Return \textbf{error}\;
         }
         Insert $\algx$ to the right of $X_{\reg,i}$\;
         \uIf{$i \ge 0$}{
             $p_{\reg} \gets p_{\reg} + 1$\;
         }
         \Else{
            $q_{\reg} \gets q_{\reg} + 1$\;
         }
    }
\end{algorithm}

\begin{algorithm}[t]
    \caption{\texttt{insert-left}$(\reg, \algx, i)$}
    \label{alg:finddelaysucc}
    
    \KwData{$\reg$: a region;
    $\algx$: the new set of clocks to insert in $\reg$;
    $i$: an index specifying the position in $\reg$ to the left of which $\algx$ is inserted;}
    \KwResult{\emph{None}, as the changes are applied directly to $\reg$.}
    \Begin() {
         \If{$(i < -q_{\reg}) \lor (i > p_{\reg})$}{
             \Return \textbf{error}\;
         }
         Insert $\algx$ to the left of $X_{\reg,i}$\;
         \uIf{$i > 0$}{
             $p_{\reg} \gets p_{\reg} + 1$\;
         }
         \Else{
            $q_{\reg} \gets q_{\reg} + 1$\;
         }
    }
\end{algorithm}

\begin{algorithm}[t]
    \caption{\texttt{remove}$(\reg, i)$}
    \label{alg:finddelaysucc}
    
    \KwData{$\reg$: a region;
    $i$: an index specifying the set $X_{\reg,i}$ to remove from $\reg$.}
    \KwResult{\emph{None}, as the changes are applied directly to $\reg$.}
    \Begin() {
         \If{$(i < -q_{\reg}) \lor (i > p_{\reg}) \lor (i = 0)$}{
             \Return \textbf{error}\;
         }
         Remove $X_{\reg, i}$ from $\reg$\;
         \uIf{$i > 0$}{
             $p_{\reg} \gets p_{\reg} - 1$\;
         }
         \Else{
            $q_{\reg} \gets q_{\reg} - 1$\;
         }
    }
\end{algorithm}

%\begin{algorithm}[H]
%    \caption{\texttt{insert-set}$(S_1, S_2)$}
%    \label{alg:copyset}
    
%    \KwData{$S_1$: a set; $S_2$: a set.}
%    \KwResult{\emph{None}, as the changes are applied directly to $S_2$.}
%    \Begin() {
%         \ForEach{$\mathit{element} \in S_1$}{
%             $S_2 \gets S_2 \cup \mathit{element}$\;
%         }
%    }
%\end{algorithm}

\begin{algorithm}[t]
    \caption{\texttt{insert-and-remove-set}$(\reg, i, j)$}
    \label{alg:insertandremove}
    
    \KwData{$\reg$: a region; 
    $i$: an integer denoting the index of the set in $\reg$ to be inserted into the set at index $j$ (after insertion, the set at index $i$ is removed from $\reg$);
    $j$: an integer denoting the index of the set in $\reg$ into which the set at index $i$ will be inserted.}
    \KwResult{\emph{None}, as the changes are applied directly to $\reg$.}
    \Begin() {
        \If{$i < -q_{\reg} \lor i > p_{\reg} \lor j < -q_{\reg} \lor j > p_{\reg} \lor i = j \lor i = 0$} {
            \Return \textbf{error}\;
        }
        \ForEach{$x \in X_{\reg, i}$}{
            $X_{\reg, j} \gets X_{\reg, j} \cup \{ x \}$\;
        }
        \texttt{remove}$(\reg, i)$\;
    }
\end{algorithm}

here we will also describe these algorithms (very briefely).
