# Supplementary material for: TARZAN: A Region-Based Library for Forward and Backward Reachability of Timed Automata (Extended Version)
Source: arXiv:2602.15435 source file (2026-02-17)
Supplement: Supplementary file 6 [file foreword_discrete_algorithm.tex]

\begin{algorithm}[tb]
    \caption{\texttt{find-discrete-successors}$(\reg)$}
    \label{alg:finddiscretesucc}
    
    \KwData{$\reg$: a region.}
    \KwResult{The set of regions reachable via discrete transitions from $\reg$.}
    
    \Begin() {
        $\mathit{res} \gets \varnothing$\; \label{line:fdsuc:initres}
        %\tcp{Get discrete transitions in the original \ac{ta} exiting from $q_{\reg}$}
        %$\mathcal{T} \gets \{ (q_{\reg}, a, \gamma, Y, q) \in T : a \in \act, \gamma \in \Gamma(\ackc), Y \subseteq \ackc, q \in Q \}$\;
        \ForEach{$t \in \{ (q_{\reg}, a, \gamma, Y, q) \in T : a \in \act, \gamma \in \Gamma(\ackc), Y \subseteq \ackc, q \in Q \}$}{ \label{line:fdsuc:foreacht}
            \If{$h_{\reg}$ satisfies $\gamma$}{ \label{line:fdsuc:isenabled}
                $\breg \gets$ copy of $\reg$\; \label{line:fdsuc:copyr}
                $q_{\breg} \gets q$\; \label{line:fdsuc:setloc}
                \For{$i = -\lidx_{\breg}$ \KwTo $\ridx_{\breg}$}{ \label{line:fdsuc:idxloop}
                    \ForEach{$x \in X_{\breg,i}$}{ \label{line:fdsuc:setloop}
                        \If{$x \in Y$}{ \label{line:fdsuc:xwasreset}
                            $h_{\breg}(x) \gets 0$\; \label{line:fdsuc:setxtozero}
                            \If{$i \neq 0$}{ \label{line:fdsuc:hasfracpart}
                                $X_{\breg,0} \gets X_{\breg,0} \cup \{x\}$;
                                $X_{\breg,i} \gets X_{\breg,i} \setminus \{x\}$\; \label{line:fdsuc:insertremovex}
                            }
                        }
                    }
                }
                % Non dovrebbe più servire togliere esplicitamente gli insiemi vuoti perchè hai già detto nella sezione 3 che gli insiemi vuoti sono omessi in automatico
                %\For{$i = -\lidx_{\breg}$ \KwTo $\ridx_{\breg}$}{
                %\If{$X_{\breg,i} = \varnothing$ and $i \neq 0$}{
                %        remove $X_{\breg, i}$ from $\breg$\;
                        %\texttt{remove}$(\breg, i)$\;
                %    }
                %}
                $\mathit{res} \gets \mathit{res} \cup \{ \breg \}$\; \label{line:fdsuc:addtores}
            }
        }
        \Return $\mathit{res}$\; \label{line:fdsuc:returnres}
    }
\end{algorithm}

\autoref{alg:finddiscretesucc} computes the immediate discrete successors of a region $\reg$.  
In particular, a set storing the resulting discrete successors is initialized in Line~\ref{line:fdsuc:initres} and returned in Line~\ref{line:fdsuc:returnres}.  
The loop in Line~\ref{line:fdsuc:foreacht} iterates over all transitions $t$ of the original \ac{ta} that exit from the current location $q_{\reg}$, identifying all possible discrete successors of $\reg$.  
If $t$ is enabled (\emph{i.e.}, its guard is satisfied by combining the integer values of the clocks, as returned by \( h_{\reg} \), with their fractional parts) (Line~\ref{line:fdsuc:isenabled}), a copy $\breg$ of $\reg$ is created to represent the successor region (Line~\ref{line:fdsuc:copyr}).  
Then, the location of $\breg$ is updated to the target location of $t$ (Line~\ref{line:fdsuc:setloc}).  
The loop in Line~\ref{line:fdsuc:idxloop} iterates over all indices of $\breg$, enabling the inner loop in Line~\ref{line:fdsuc:setloop} to examine each clock set of $\breg$.  
If a clock $x$ is reset by $t$ (Line~\ref{line:fdsuc:xwasreset}), its integer value is set to zero (Line~\ref{line:fdsuc:setxtozero}).  
Moreover, if $x$ has a non-zero fractional part (Line~\ref{line:fdsuc:hasfracpart}), it is inserted into $X_{\breg, 0}$ and removed from its previous set (Line~\ref{line:fdsuc:insertremovex}).  
Finally, the resulting region $\breg$ is added to the result set in Line~\ref{line:fdsuc:addtores}.
