# Supplementary material for: TARZAN: A Region-Based Library for Forward and Backward Reachability of Timed Automata (Extended Version)
Source: arXiv:2602.15435 source file (2026-02-17)
Supplement: Supplementary file 7 [file perm-regs.tex]

\autoref{alg:perm-regs} computes all regions derived from the input region $\reg$ by finding all ordered partitions of a clock set $X$, while preserving the relative order of predefined \Blue{clock sets} $X_{\reg,i}, \dots, X_{\reg,j}$ (where $i \leq j$). 
For each resulting region, the integer value of every clock $x$ is given by $\mathcal{H}(x)$.

In particular,
