# Supplementary material for: TARZAN: A Region-Based Library for Forward and Backward Reachability of Timed Automata (Extended Version)
Source: arXiv:2602.15435 source file (2026-02-17)
Supplement: Supplementary file 8 [file production_cell_appendix.tex]

\begin{figure}[ht]
\begin{center}
\begin{tikzpicture}[
	->,
	>=stealth',
	shorten >=2pt, 
	auto,
    transform shape,
    align=center,
    scale=0.77,
    state/.style={thick, circle, draw, minimum size=1.3cm}
    ] 
    
    \node[
          state,
          accepting
          %initial,
          %initial text =
          %label=above left:$\mathbf{c}$
         ] 
         (q0) {$\mathit{feed}$};
	
    \node[
          state,
          %label=above left:$\mathbf{c}$,
          right = 4.6cm of q0
         ] 
         (q1) {$\mathit{table}$};
	
    \node[
          state,
          %label=above left:$\mathbf{c}$,
          right = 4.6cm of q1
         ] 
         (q2) {$\mathit{robot_p}$};

    \node[
          state,
          %label=above left:$\mathbf{c}$,
          above = 2.8cm of q2
         ] 
         (q3) {$\mathit{press}$};
	
    \node[
          state,
          %label=above left:$\mathbf{c}$,
          left = 4.6cm of q3
         ] 
         (q4) {$\mathit{robot_d}$};
	
    \node[
          state,
          %label=above left:$\mathbf{c}$,
          left = 4.6cm of q4
         ] 
         (q5) {$\mathit{depot}$};

    \node[
          state,
          rectangle,
          minimum size=1.2cm,
          %label=above left:$\mathbf{e}$,
          left = 0cm of q2,
          yshift=2.7cm
         ] 
         (q6) {$\mathit{fall_p}$};

    \node[
          state,
          rectangle,
          minimum size=1.2cm,
          %label=above left:$\mathbf{e}$,
          right = 0cm of q0,
          yshift=2.7cm
         ] 
         (q7) {$\mathit{fall_d}$};

	\draw [thick] 
    
	(q0) 
    edge 
    node[above, pos=0.6]{$\mathit{toTable}$ \\ $x = 2$} 
    node[below, pos=0.6]{$\resetClock{x}$}
    (q1)
	
    (q1) 
    edge 
    node[above, pos=0.4]{$\mathit{takePlate_p}$ \\ $x \ge 1 \land x \le 3$} 
    node[below, pos=0.4]{$\resetClock{x}$}
    (q2)

    (q2) 
    edge 
    node[right]{$\mathit{toPress}$ \\ $x \ge 2 \land x \le 4$ \\ $\resetClock{x}$}
    (q3)

    (q3) 
    edge 
    node[above]{$\mathit{takePlate_d}$ \\ $x \ge 3 \land x \le 5$} 
    node[below]{$\resetClock{x}$}
    (q4)

    (q4) 
    edge 
    node[above]{$\mathit{toDepot}$ \\ $x \ge 3 \land x \le 6 \land y \le 30$} 
    node[below]{$\resetClock{x}$}
    (q5)

    (q2) 
    edge 
    node[left, yshift=-7pt, xshift=-3pt]{$\mathit{toPress}$ \\ $x < 2$ \\ $\resetClock{x}$}
    (q6)

    (q4) 
    edge %[out=270, in=0]
    node[right, pos=0.4, xshift = -12pt, yshift=-20pt]{$\mathit{toDepot}$ \\ $x \ge 4$ \\ $\resetClock{x}$}
    (q7)

    (q6) 
    edge [out=180, in=15]
    node[right, pos=0.5, xshift=22pt]{$\mathit{restore_p}$ \\ $x > 1 \land x < 2$}
    (q0)

    (q7) 
    edge
    node[right, pos=0.4, xshift=-2pt]{$\mathit{restore_d}$ \\ $x > 1 \land x \le 5$}
    (q0)

    (q5) 
    edge 
    node[left]{ $\mathit{newPlate}$ \\ $\resetClock{x}$}
    (q0)
	;
\end{tikzpicture}
\end{center}
\caption{A \ac{ta} modeling a Production Cell.
The passage of time is tracked by clock $y$.}
\label{fig:production_cell}
\end{figure}
