# Supplementary material for: TARZAN: A Region-Based Library for Forward and Backward Reachability of Timed Automata (Extended Version)
Source: arXiv:2602.15435 source file (2026-02-17)
Supplement: Supplementary file 9 [file timed_games_example_appendix.tex]

A \ac{ta} modeling a Production Cell~\cite{Burns2003} (referred to as Cell for brevity) is depicted in \autoref{fig:production_cell}.
A Timed Game can be defined over the Cell, where two players, the \emph{controller} and the \emph{environment}, interact by making choices over time. 
The Cell’s locations are partitioned into controller and environment locations represented, respectively, as circles and squares.
Players move as follows: the controller begins by selecting an action to perform. Depending on the current location type (either circle or square), it is either the controller or the environment who then chooses a delay before the action takes effect.
Once the action and the delay have been determined, the environment finally chooses which Cell transition, compatible with the chosen action and delay, is executed.

The Cell operates by retrieving metal plates transported from a feed belt ($\mathit{feed}$) to a rotary table ($\mathit{table}$), pressing them ($\mathit{press}$), and subsequently storing them in a depot ($\mathit{depot}$). 
Plates are transported between different stations by a two-armed robot, where arm $P$ ($\mathit{robot_p}$) picks up plates from the table and places them onto the press, while arm $D$ ($\mathit{robot_d}$) transfers the pressed plates into the depot.
If the robot moves too quickly or holds plates for too long, they may fall to the ground ($\mathit{fall_p}$ and $\mathit{fall_d}$) and must be placed onto the feed belt to start the process again.
The time required to put fallen plates onto the feed belt is not under the control of the Cell.

\begin{figure}[ht]
\begin{center}
\begin{tikzpicture}[
	->,
	>=stealth',
	shorten >=2pt, 
	auto,
    transform shape,
    align=center,
    scale=0.77,
    state/.style={thick, circle, draw, minimum size=1.3cm}
    ] 
    
    \node[
          state,
          accepting
          %initial,
          %initial text =
          %label=above left:$\mathbf{c}$
         ] 
         (q0) {$\mathit{feed}$};
	
    \node[
          state,
          %label=above left:$\mathbf{c}$,
          right = 4.6cm of q0
         ] 
         (q1) {$\mathit{table}$};
	
    \node[
          state,
          %label=above left:$\mathbf{c}$,
          right = 4.6cm of q1
         ] 
         (q2) {$\mathit{robot_p}$};

    \node[
          state,
          %label=above left:$\mathbf{c}$,
          above = 2.8cm of q2
         ] 
         (q3) {$\mathit{press}$};
	
    \node[
          state,
          %label=above left:$\mathbf{c}$,
          left = 4.6cm of q3
         ] 
         (q4) {$\mathit{robot_d}$};
	
    \node[
          state,
          %label=above left:$\mathbf{c}$,
          left = 4.6cm of q4
         ] 
         (q5) {$\mathit{depot}$};

    \node[
          state,
          rectangle,
          minimum size=1.2cm,
          %label=above left:$\mathbf{e}$,
          left = 0cm of q2,
          yshift=2.7cm
         ] 
         (q6) {$\mathit{fall_p}$};

    \node[
          state,
          rectangle,
          minimum size=1.2cm,
          %label=above left:$\mathbf{e}$,
          right = 0cm of q0,
          yshift=2.7cm
         ] 
         (q7) {$\mathit{fall_d}$};

	\draw [thick] 
    
	(q0) 
    edge 
    node[above, pos=0.6]{$\mathit{toTable}$ \\ $x = 2$} 
    node[below, pos=0.6]{$\resetClock{x}$}
    (q1)
	
    (q1) 
    edge 
    node[above, pos=0.4]{$\mathit{takePlate_p}$ \\ $x \ge 1 \land x \le 3$} 
    node[below, pos=0.4]{$\resetClock{x}$}
    (q2)

    (q2) 
    edge 
    node[right]{$\mathit{toPress}$ \\ $x \ge 2 \land x \le 4$ \\ $\resetClock{x}$}
    (q3)

    (q3) 
    edge 
    node[above]{$\mathit{takePlate_d}$ \\ $x \ge 3 \land x \le 5$} 
    node[below]{$\resetClock{x}$}
    (q4)

    (q4) 
    edge 
    node[above]{$\mathit{toDepot}$ \\ $x \ge 3 \land x \le 6 \land y \le 30$} 
    node[below]{$\resetClock{x}$}
    (q5)

    (q2) 
    edge 
    node[left, yshift=-7pt, xshift=-3pt]{$\mathit{toPress}$ \\ $x < 2$ \\ $\resetClock{x}$}
    (q6)

    (q4) 
    edge %[out=270, in=0]
    node[right, pos=0.4, xshift = -12pt, yshift=-20pt]{$\mathit{toDepot}$ \\ $x \ge 4$ \\ $\resetClock{x}$}
    (q7)

    (q6) 
    edge [out=180, in=15]
    node[right, pos=0.5, xshift=22pt]{$\mathit{restore_p}$ \\ $x > 1 \land x < 2$}
    (q0)

    (q7) 
    edge
    node[right, pos=0.4, xshift=-2pt]{$\mathit{restore_d}$ \\ $x > 1 \land x \le 5$}
    (q0)

    (q5) 
    edge 
    node[left]{ $\mathit{newPlate}$ \\ $\resetClock{x}$}
    (q0)
	;
\end{tikzpicture}
\end{center}
\caption{A \ac{ta} modeling a Production Cell.
The passage of time is tracked by clock $y$.}
\label{fig:production_cell}
\end{figure}

%\autoref{alg:finddelaypred} and \autoref{alg:finddiscretepred} can be used to solve such a game. 
Let us assume that the controller must reach location $\mathit{depot}$ starting from $\mathit{feed}$ within $30$ time units (as enforced by the clock constraint $y \leq 30$ on the transition entering $\mathit{depot}$), while visiting only controller locations.
To determine whether the controller has a winning strategy, it is possible to apply a fixed-point backward reachability algorithm. 
Classical algorithms, such as those presented in~\cite{ASARIN1998447} and~\cite[Chapter 9]{GoG}, can be easily adapted to this setting.
The computation begins from the goal regions, \emph{i.e.}, those located in $\mathit{depot}$ satisfying $y \leq 30$ and iteratively applies delay and discrete predecessor computations by using \autoref{alg:finddelaypred} and \autoref{alg:finddiscretepred} until a region in $\mathit{feed}$ is reached where both $x = 0$ and $y = 0$ hold ($x$ and $y$ are initialized to $0$ at the start of the Cell execution). 
Notice that each region traversed by the fixed-point backward reachability algorithm must guarantee the controller’s victory.

%To compute a winning strategy, a backward reachability algorithm can be employed, starting from the set of goal regions, \emph{i.e.}, those located in $\mathit{depot}$ and satisfying the timing constraint $27 \le y \le 30$. 
%This set is finite and relatively small given the the restricted range of allowed values for $x$ and $y$. 
%The algorithm then computes delay and discrete predecessor regions using \autoref{alg:finddelaypred} and \autoref{alg:finddiscretepred} until it reaches a region in $\mathit{feed}$ where both $x = 0$ and $y = 0$ hold ($x$ and $y$ are initialized to 0 at the beginning of the Cell execution).
%It is worth noticing that every transition originating from a controller location resets only clock $x$ and clock $x$ appears in non strict guards, which remains bounded throughout the entire Cell execution, since only controller locations must be visited by the controller. 
%This mitigates the exponential blow-up of \autoref{alg:finddiscretepred}.
