# Supplementary material for: TARZAN: A Region-Based Library for Forward and Backward Reachability of Timed Automata (Extended Version)
Source: arXiv:2602.15435 source file (2026-02-17)
Supplement: Supplementary file 11 [file alltoghether.tex]

\begin{figure}[tb]
\centering
\begin{subfigure}{0.34\textwidth}
  \centering
  \begin{tikzpicture}[
    ->,
    >=stealth',
    shorten >=2pt, 
    auto,
    transform shape,
    align=center,
    scale=0.865,
    state/.style={thick, circle, draw, minimum size=1cm}
] 
\useasboundingbox (-1.9, -3.1) rectangle (2.7, 1.71);

  % Main state
  \node[state, accepting] (q) {$q_0$};
  % Goal state below
  \node[state, below of=q, yshift=-1.5cm] (goal) {$\mathit{Goal}$};
  % Ellipsis to suggest more loops (slightly above q)
  \node[above=1cm of q, xshift=23pt, yshift=-37pt] (dots) {\Large $\mathbf{\cdots}$};
  \draw [thick] 
  % Edges and loops
  (q) edge[loop, in=180, out=240, looseness=8]  node[below, xshift=0pt, yshift=-6pt]  {$x_1 = 1$ \\ $\resetClock{x_1}$} (q)
  
  (q) edge[loop, in=90, out=150, looseness=8] node[right, xshift=21pt, yshift=0pt] {$x_2 = 2$ \\ $\resetClock{x_2}$} (q)
  
  (q) edge[loop, in=300, out=0, looseness=8] node[right, xshift=1pt, yshift=5pt] {$x_n = n$ \\ $\resetClock{x_n}$} (q)
  
  (q) edge node[right, yshift=-13pt] {$x_1 = \cdots = x_n = 0$ \\ $\land \; y \geq 1$} (goal);

  %\draw[red, thick, dashed] (current bounding box.south west) rectangle (current bounding box.north east);
\end{tikzpicture}
  \caption{\flower{}.}
  \label{fig:flower_sub}
\end{subfigure}
\hfill
\begin{subfigure}{0.3\textwidth}
  \centering
  \begin{tikzpicture}[
    ->,
    >=stealth',
    shorten >=2pt, 
    auto,
    transform shape,
    align=center,
    scale=0.865,
    state/.style={thick, circle, draw, minimum size=1cm}
] 
%\useasboundingbox (-2, -3.1) rectangle (2.9, 1.71);

  \node[state, accepting] (q) {$q_0$};
  \node[state, right=2cm of q] (q1) {$q_1$};
  
  \draw [thick] 
  % Edges and loops
  (q) edge[in=150, out=30]  
  node[xshift=0pt, yshift=0pt]  
  {$x_i = i$ \\ $\mathbf{x}_{\boldsymbol{i}} \boldsymbol{:=} \mathbf{0}, \boldsymbol{ctr_i} \boldsymbol{:=} \mathbf{1} \mathbf{-} \boldsymbol{ctr_i}$} (q1)

  (q1) edge[in=330, out=210]  
  node[xshift=0pt, yshift=0pt]  
  {$x_i = i$ \\ $\mathbf{x}_{\boldsymbol{i}} \boldsymbol{:=} \mathbf{0}, \boldsymbol{ctr_i} \boldsymbol{:=} \mathbf{1} \mathbf{-} \boldsymbol{ctr_i}$} (q);

  %\draw[red, thick, dashed] (current bounding box.south west) rectangle (current bounding box.north east);
\end{tikzpicture}
  \caption{\boolea{}.}
  \label{fig:boolean_sub}
\end{subfigure}
\hfill
\begin{subfigure}{0.3\textwidth}
  \centering
  \begin{tikzpicture}[
    ->,
    >=stealth',
    shorten >=2pt, 
    auto,
    transform shape,
    align=center,
    scale=0.865,
    state/.style={thick, circle, draw, minimum size=1cm}
] 
 
  \node[state, accepting] (q) {$q_0$};
  \node[state, right=2cm of q] (q1) {$q_1$};
  \node[state, below=1.2cm of q1] (q2) {$q_4$};
  \node[state, left=2cm of q2] (q3) {$\mathit{Goal}$};
  
  \draw[thick, ->] (q) --  node[above] {$x_i = i$ \\ $\mathbf{x}_{\boldsymbol{i}} \boldsymbol{:=} \mathbf{0}$} (q1);
  \draw[thick, -] (q1) -- ($(q1)!0.35!(q2)$);
  \draw[thick, dashed, -] ($(q1)!0.35!(q2)$) -- ($(q1)!0.55!(q2)$);
  \draw[thick, ->] ($(q1)!0.55!(q2)$) -- (q2);
  \draw[thick, ->] (q2) --  node[below] {$x_i = i$ \\ $\mathbf{x}_{\boldsymbol{i}} \boldsymbol{:=} \mathbf{0}$} (q3);
  \draw[thick, ->] (q3) --  node[right] {$x_i = i$ \\ $\mathbf{x}_{\boldsymbol{i}} \boldsymbol{:=} \mathbf{0}$} (q);

   %\draw[red, thick, dashed] (current bounding box.south west) rectangle (current bounding box.north east);
\end{tikzpicture}
  \caption{\ring{}.}
  \label{fig:ring_sub}
\end{subfigure}

% Add vertical space and start second row
\vspace{1.5em}  % Adjust spacing as needed

% Second row - centered
\begin{subfigure}{\textwidth}
  \centering
  \begin{tikzpicture}[
    ->,
    >=stealth',
    shorten >=2pt, 
    auto,
    transform shape,
    align=center,
    scale=0.865,
    state/.style={thick, circle, draw, minimum size=1cm}
] 
 
  % First row
  \node[state, accepting] (q) {$q_0$};
  \node[state, left=0.1cm of q, draw=none] (k) {$\mathit{Key}_i$};
  \node[state, right=2cm of q] (q1) {$q_1$};
  \node[state, right=2cm of q1] (q2) {$q_{i-1}$};
  \node[state, right=2cm of q2] (q3) {$q_i$};
  
  % Edges for first row
  \draw[thick, ->] (q) --  node[below] {$x_i = i$ \\ $\mathbf{x}_{\boldsymbol{i}} \boldsymbol{:=} \mathbf{0}$} (q1);
  \draw[thick, -] (q1) -- ($(q1)!0.3!(q2)$);
  \draw[thick, dashed, -] ($(q1)!0.3!(q2)$) -- ($(q1)!0.61!(q2)$);
  \draw[thick, ->] ($(q1)!0.61!(q2)$) -- (q2);
  \draw[thick, ->] (q2) --  node[below] {$x_i = i$ \\ $\boldsymbol{gate} \boldsymbol{:=} \boldsymbol{gate} \mathbf{+} \mathbf{1}$} (q3);
  
  % Second row (below first)
  \node[state, accepting, below=0.6cm of q] (p) {$q_0$};
  \node[state, left=0.1cm of p, draw=none] (u) {$\mathit{Unlocker}$};
  \node[state, right=2cm of p] (p1) {$q_1$};
  \node[state, right=2cm of p1] (p2) {$q_{K - 1}$};
  \node[state, right=2cm of p2] (p3) {$\mathit{Goal}$};
  
  % Edges for second row
  \draw[thick, ->] (p) --  node[below] {$x = K - 1$ \\ $\resetClock{x}$} (p1);
  \draw[thick, -] (p1) -- ($(p1)!0.3!(p2)$);
  \draw[thick, dashed, -] ($(p1)!0.3!(p2)$) -- ($(p1)!0.61!(p2)$);
  \draw[thick, ->] ($(p1)!0.61!(p2)$) -- (p2);
  \draw[thick, ->] (p2) --  node[below] {$x = K - 1$ \\ $\land \; \mathit{gate} = K - 1$} (p3);

   %\draw[red, thick, dashed] (current bounding box.south west) rectangle (current bounding box.north east);
   
\end{tikzpicture}
  \caption{\gates{}.}
  \label{fig:gates_sub}
\end{subfigure}

\caption{Depiction of the benchmark \ac{ta} used in both \autoref{tab:punctual} and \autoref{tab:punctual_full}.
\boolea{}, \ring{}, and \gates{} are manually constructed networks of \ac{ta}, whereas \flower{} is a single \ac{ta} adapted from~\cite{J_rgensen_2012} (it is included here for completeness).}
\label{fig:overall}
\end{figure}
