# Supplementary material for: TARZAN: A Region-Based Library for Forward and Backward Reachability of Timed Automata (Extended Version)
Source: arXiv:2602.15435 source file (2026-02-17)
Supplement: Supplementary file 26 [file full_state_space_full.tex]

\definecolor{lightgray}{gray}{0.95}
\setlength{\aboverulesep}{1pt}
\setlength{\belowrulesep}{1pt}
{
{\setlength{\tabcolsep}{3.25pt}
\begin{table}[tb]
\centering
\caption{Safety properties require \toolname{} to visit the entire reachable state space.}
\label{tab:full_state_space_full}
\resizebox{\textwidth}{!}{
\begin{tabular}{%
    c|rrrr|rrrr|rrrr
}
\toprule
\multirow{2}{*}{\textbf{K}}
  & \multicolumn{4}{c|}{\textbf{TARZAN}}
  & \multicolumn{4}{c|}{\textbf{TChecker}}
  & \multicolumn{4}{c}{\textbf{UPPAAL}} \\
  & \multicolumn{1}{c}{\textbf{VT}}
  & \multicolumn{1}{c}{\textbf{ET}}
  & \multicolumn{1}{c}{\textbf{Mem}}
  & \multicolumn{1}{c|}{\textbf{Regions}}
  & \multicolumn{1}{c}{\textbf{VT}}
  & \multicolumn{1}{c}{\textbf{ET}}
  & \multicolumn{1}{c}{\textbf{Mem}}
  & \multicolumn{1}{c|}{\textbf{States}}
  & \multicolumn{1}{c}{\textbf{VT}}
  & \multicolumn{1}{c}{\textbf{ET}}
  & \multicolumn{1}{c}{\textbf{Mem}}
  & \multicolumn{1}{c}{\textbf{States}} \\
\midrule
% ----------------------- FISCHER DATASET -----------------------
\multicolumn{13}{c}{$\blacktriangleright$
{\normalsize \fischer{}}~\cite{uppaalSite} ::
[Query: $\exists \Diamond ( \mathit{Fischer}_1.\mathit{cs} \land \mathit{Fischer}_2.\mathit{cs} ) $]
$\blacktriangleleft$} \\
\midrule
\rowcolor{white}
2  & 0.001 & 0.015 & 9.60 & 542
   & ${\boldsymbol \varepsilon}$ & \textbf{0.006} & \textbf{6.01} & \textbf{18}
   & 0.001 & 0.055 & 18.87 & 18 \\
\rowcolor{lightgray}
3  & 0.025 & 0.039 & 55.62 & 9324
   & ${\boldsymbol \varepsilon}$ & \textbf{0.006} & \textbf{6.26} & \textbf{65}
   & 0.001 & 0.055 & 18.91 & 65 \\
\rowcolor{white}
4  & 0.644 & 0.669 & 1098.36 & 180032
   & ${\boldsymbol \varepsilon}$ & \textbf{0.007} & \textbf{6.75} & \textbf{220}
   & 0.001 & 0.055 & 18.96 & 220 \\
\rowcolor{lightgray}
5  & 19.627 & 19.849 & 12948.99 & 3920652
   & 0.004 & 0.011 & 9.30 & 727
   & \textbf{0.002} & \textbf{0.057} & \textbf{19.07} & \textbf{727} \\
\rowcolor{white}
6  & --- & --- & OOM & ---
   & 0.024 & 0.032 & 12.25 & 2378
   & \textbf{0.008} & \textbf{0.064} & \textbf{19.43} & \textbf{2378} \\
\midrule
% ----------------------- LYNCH DATASET -----------------------
\multicolumn{13}{c}{$\blacktriangleright$
{\normalsize \lynch{}}~\cite{farkas2018towards} ::
[Query: $\exists \Diamond ( P_1.\mathit{CS}7 \land P_2.\mathit{CS}7 ) $]
$\blacktriangleleft$} \\
\midrule
\rowcolor{white}
2  & 0.076 & 0.091 & 152.12 & 32268
   & ${\boldsymbol \varepsilon}$ & \textbf{0.007} & \textbf{6.19} & \textbf{38}
   & $\varepsilon$ & 0.058 & 18.95 & 38 \\
\rowcolor{lightgray}
3  & 20.137 & 20.373 & 12857.20 & 5289449
   & ${\boldsymbol \varepsilon}$ & \textbf{0.008} & \textbf{6.49} & \textbf{125}
   & 0.001 & 0.056 & 19.05 & 125 \\
\rowcolor{white}
4  & --- & --- & OOM & ---
   & \textbf{0.001} & \textbf{0.010} & \textbf{7.38} & \textbf{380}
   & 0.001 & 0.057 & 19.15 & 380 \\
\bottomrule
\end{tabular}
}
\end{table}
}
}
