# Supplementary material for: TARZAN: A Region-Based Library for Forward and Backward Reachability of Timed Automata (Extended Version)
Source: arXiv:2602.15435 source file (2026-02-17)
Supplement: Supplementary file 27 [file others.tex]

\definecolor{lightgray}{gray}{0.95}
\setlength{\aboverulesep}{1pt}
\setlength{\belowrulesep}{1pt}
{
{\setlength{\tabcolsep}{3.25pt}
\begin{table}[tb]
\centering
\caption{In small to medium-sized benchmarks, regions perform comparably with zones.
Here, \exSITH{} and \simple{} are single \ac{ta}.}
\label{tab:others}
\resizebox{\textwidth}{!}{
\begin{tabular}{%
    c|rrrr|rrrr|rrrr
}
\toprule
\multirow{2}{*}{\textbf{K}}
  & \multicolumn{4}{c|}{\textbf{TARZAN}}
  & \multicolumn{4}{c|}{\textbf{TChecker}}
  & \multicolumn{4}{c}{\textbf{UPPAAL}} \\
  & \multicolumn{1}{c}{\textbf{VT}}
  & \multicolumn{1}{c}{\textbf{ET}}
  & \multicolumn{1}{c}{\textbf{Mem}}
  & \multicolumn{1}{c|}{\textbf{Regions}}
  & \multicolumn{1}{c}{\textbf{VT}}
  & \multicolumn{1}{c}{\textbf{ET}}
  & \multicolumn{1}{c}{\textbf{Mem}}
  & \multicolumn{1}{c|}{\textbf{States}}
  & \multicolumn{1}{c}{\textbf{VT}}
  & \multicolumn{1}{c}{\textbf{ET}}
  & \multicolumn{1}{c}{\textbf{Mem}}
  & \multicolumn{1}{c}{\textbf{States}} \\
\midrule
% ----------------------- ANDORORIGINAL DATASET -----------------------
\multicolumn{13}{c}{$\blacktriangleright$
{\normalsize \andor{}}~\cite{farkas2018towards} ::
[Query: $\exists \Diamond ( \mathit{false} ) $]
$\blacktriangleleft$} \\
\midrule
\rowcolor{white}
3  & 0.001 & 0.016 & 14.50 & 640
   & ${\boldsymbol \varepsilon}$ & \textbf{0.007} & \textbf{6.35} & \textbf{9}
   & $\varepsilon$ & 0.052 & 18.96 & 8 \\
\midrule
% ----------------------- EXSITH DATASET -----------------------
\multicolumn{13}{c}{$\blacktriangleright$
{\normalsize \exSITH{}}~\cite{farkas2018towards} ::
[Query: $\exists \Diamond ( A.\mathit{qBad} ) $]
$\blacktriangleleft$} \\
\midrule
\rowcolor{white}
1  & $\varepsilon$ & 0.013 & 8.10 & 225
   & ${\boldsymbol \varepsilon}$ & \textbf{0.006} & \textbf{5.87} & \textbf{4}
   & $\varepsilon$ & 0.054 & 18.79 & 4 \\
\midrule
% ----------------------- LATCH DATASET -----------------------
\multicolumn{13}{c}{$\blacktriangleright$
{\normalsize \latch{}}~\cite{farkas2018towards} ::
[Query: $\exists \Diamond ( \mathit{Latch}_1.\mathit{LatchD1E1} ) $]
$\blacktriangleleft$} \\
\midrule
\rowcolor{white}
7  & 0.009 & 0.024 & 59.34 & 2025
   & ${\boldsymbol \varepsilon}$ & \textbf{0.008} & \textbf{6.36} & \textbf{7}
   & $\varepsilon$ & 0.056 & 19.03 & 7 \\
\midrule
% ----------------------- MALER DATASET -----------------------
\multicolumn{13}{c}{$\blacktriangleright$
{\normalsize \maler{}}~\cite{farkas2018towards} ::
[Query: $\exists \Diamond ( \mathit{Job}_1.\mathit{End}1 \land \mathit{Job}_2.\mathit{End}2 \land \mathit{Job}_3.\mathit{End}3 \land \mathit{Job}_4.\mathit{End}4 ) $]
$\blacktriangleleft$} \\
\midrule
\rowcolor{white}
4  & $\varepsilon$ & 0.014 & 8.38 & 114
   & ${\boldsymbol \varepsilon}$ & \textbf{0.008} & \textbf{6.35} & \textbf{75}
   & $\varepsilon$ & 0.056 & 19.11 & 75 \\
\midrule
% ----------------------- RCP DATASET -----------------------
\multicolumn{13}{c}{$\blacktriangleright$
{\normalsize \rcp{}}~\cite{farkas2018towards} ::
[Query: $\exists \Diamond ( \mathit{S1o.S1oEnd} ) $]
$\blacktriangleleft$} \\
\midrule
\rowcolor{white}
5  & 0.001 & 0.014 & 12.25 & 346
   & ${\boldsymbol \varepsilon}$ & \textbf{0.010} & \textbf{6.50} & \textbf{27}
   & 0.001 & 0.056 & 19.18 & 18 \\
\midrule
% ----------------------- SIMPLE DATASET -----------------------
\multicolumn{13}{c}{$\blacktriangleright$
{\normalsize \simple{}}~\cite{jensen2023dynamic} ::
[Query: $\exists \Diamond ( \mathit{false} ) $]
$\blacktriangleleft$} \\
\midrule
\rowcolor{white}
1  & $\varepsilon$ & 0.013 & 7.64 & 56
   & ${\boldsymbol \varepsilon}$ & \textbf{0.006} & \textbf{5.81} & \textbf{3}
   & $\varepsilon$ & 0.053 & 18.76 & 3 \\
\rowcolor{lightgray}
1  & $\varepsilon$ & 0.013 & 7.92 & 428
   & ${\boldsymbol \varepsilon}$ & \textbf{0.006} & \textbf{5.90} & \textbf{3}
   & $\varepsilon$ & 0.054 & 18.76 & 3 \\
\rowcolor{white}
1  & 0.001 & 0.015 & 12.28 & 4028
   & \textbf{0.001} & \textbf{0.007} & \textbf{6.52} & \textbf{3}
   & 0.001 & 0.054 & 18.83 & 3 \\
\midrule
% ----------------------- SOLDIERS DATASET -----------------------
\multicolumn{13}{c}{$\blacktriangleright$
{\normalsize \soldiers{}}~\cite{farkas2018towards} ::
[Query: $\exists \Diamond ( E.\mathit{Escape} ) $]
$\blacktriangleleft$} \\
\midrule
\rowcolor{white}
5  & 0.128 & 0.146 & 494.43 & 24194
   & ${\boldsymbol \varepsilon}$ & \textbf{0.007} & \textbf{6.45} & \textbf{93}
   & $\varepsilon$ & 0.056 & 19.05 & 93 \\
\midrule
% ----------------------- SRLATCH DATASET -----------------------
\multicolumn{13}{c}{$\blacktriangleright$
{\normalsize \srlatch{}}~\cite{farkas2018towards} ::
[Query: $\exists \Diamond ( \mathit{Env.envFinal} ) $]
$\blacktriangleleft$} \\
\midrule
\rowcolor{white}
3  & $\varepsilon$ & 0.013 & 7.62 & 9
   & ${\boldsymbol \varepsilon}$ & \textbf{0.007} & \textbf{6.24} & \textbf{5}
   & $\varepsilon$ & 0.052 & 19.05 & 4 \\
\bottomrule
\end{tabular}
}
\end{table}
}
}
