# Supplementary material for: TARZAN: A Region-Based Library for Forward and Backward Reachability of Timed Automata (Extended Version)
Source: arXiv:2602.15435 source file (2026-02-17)
Supplement: Supplementary file 28 [file punctual_guards_full.tex]

\definecolor{lightgray}{gray}{0.95}
\setlength{\aboverulesep}{1pt}
\setlength{\belowrulesep}{1pt}
{
{\setlength{\tabcolsep}{3.25pt}
\begin{table}[tb]
\centering
\caption{When all transitions have punctual guards, regions may outperform zones.
Here, \flower{} is a single \ac{ta}, while the others are networks of \ac{ta}.}
\label{tab:punctual_full}
\resizebox{\textwidth}{!}{
\begin{tabular}{%
    c|rrrr|rrrr|rrrr
}
\toprule
\multirow{2}{*}{\textbf{K}}
  & \multicolumn{4}{c|}{\textbf{TARZAN}}
  & \multicolumn{4}{c|}{\textbf{TChecker}}
  & \multicolumn{4}{c}{\textbf{UPPAAL}} \\
  & \multicolumn{1}{c}{\textbf{VT}}
  & \multicolumn{1}{c}{\textbf{ET}}
  & \multicolumn{1}{c}{\textbf{Mem}}
  & \multicolumn{1}{c|}{\textbf{Regions}}
  & \multicolumn{1}{c}{\textbf{VT}}
  & \multicolumn{1}{c}{\textbf{ET}}
  & \multicolumn{1}{c}{\textbf{Mem}}
  & \multicolumn{1}{c|}{\textbf{States}}
  & \multicolumn{1}{c}{\textbf{VT}}
  & \multicolumn{1}{c}{\textbf{ET}}
  & \multicolumn{1}{c}{\textbf{Mem}}
  & \multicolumn{1}{c}{\textbf{States}} \\
\midrule
% ----------------------- BOOLEAN DATASET -----------------------
\multicolumn{13}{c}{$\blacktriangleright$
{\normalsize \boolea{}}~\cite{tarzan2025} ::
[Query: $\exists \Diamond( \mathit{ctr}_1 = 1 \land \mathit{ctr}_2 = 1 \land \dots \land \mathit{ctr}_K = 1 )$]
$\blacktriangleleft$} \\
\midrule
\rowcolor{white}
2  & $\varepsilon$ & 0.013 & 7.62 & 9
   & ${\boldsymbol \varepsilon}$ & \textbf{0.005} & \textbf{5.92} & \textbf{6}
   & $\varepsilon$ & 0.051 & 18.80 & 6 \\
\rowcolor{lightgray}
4  & $\varepsilon$ & 0.013 & 7.78 & 24
   & ${\boldsymbol \varepsilon}$ & \textbf{0.007} & \textbf{6.47} & \textbf{185}
   & 0.001 & 0.052 & 18.85 & 185 \\
\rowcolor{white}
6  & \textbf{0.003} & \textbf{0.016} & \textbf{13.42} & \textbf{425}
   & 0.088 & 0.096 & 13.80 & 8502
   & 0.075 & 0.128 & 19.91 & 8502 \\
\rowcolor{lightgray}
8  & \textbf{0.013} & \textbf{0.027} & \textbf{29.10} & \textbf{1009}
   & 75.461 & 75.980 & 220.82 & 566763
   & 77.204 & 77.523 & 81.79 & 566763 \\
\rowcolor{white}
10  & \textbf{0.070} & \textbf{0.086} & \textbf{110.29} & \textbf{4050}
   & --- & TO & --- & ---
   & --- & TO & --- & --- \\
\rowcolor{lightgray}
12  & \textbf{0.341} & \textbf{0.361} & \textbf{476.73} & \textbf{15961}
   & --- & TO & --- & ---
   & --- & TO & --- & --- \\
\rowcolor{white}
14  & \textbf{0.737} & \textbf{0.764} & \textbf{965.29} & \textbf{28679}
   & --- & TO & --- & ---
   & --- & TO & --- & --- \\
\rowcolor{lightgray}
16  & \textbf{1.578} & \textbf{1.616} & \textbf{1788.46} & \textbf{43919}
   & --- & TO & --- & ---
   & --- & TO & --- & --- \\
\midrule
% ----------------------- FLOWER DATASET -----------------------
\multicolumn{13}{c}{$\blacktriangleright$
{\normalsize \flower{}}~\cite{J_rgensen_2012} :: 
[Query: $\exists \Diamond ( \mathit{Flower.Goal} )$]
$\blacktriangleleft$} \\
\midrule
\rowcolor{white}
3  & $\varepsilon$ & 0.013 & 7.64 & 13
   & ${\boldsymbol \varepsilon}$ & \textbf{0.005} & \textbf{5.84} & \textbf{7}
   & $\varepsilon$ & 0.055 & 18.80 & 7 \\
\rowcolor{lightgray}
5  & ${\boldsymbol \varepsilon}$ & \textbf{0.013} & \textbf{7.92} & \textbf{95}
   & 0.001 & 0.007 & 6.35 & 150
   & 0.001 & 0.056 & 18.82 & 150 \\
\rowcolor{white}
7  & ${\boldsymbol \varepsilon}$ & \textbf{0.022} & \textbf{10.65} & \textbf{573}
   & 0.322 & 0.330 & 13.12 & 3508
   & 0.399 & 0.455 & 19.76 & 3508 \\
\rowcolor{lightgray}
9  & \textbf{0.007} & \textbf{0.022} & \textbf{58.62} & \textbf{9161}
   & --- & TO & --- & ---
   & --- & TO & --- & --- \\
\rowcolor{white}
11  & \textbf{0.028} & \textbf{0.044} & \textbf{177.34} & \textbf{30761}
   & --- & TO & --- & ---
   & --- & TO & --- & --- \\
\rowcolor{lightgray}
13  & \textbf{0.412} & \textbf{0.450} & \textbf{2034.18} & \textbf{370331}
   & --- & TO & --- & ---
   & --- & TO & --- & --- \\
\rowcolor{white}
15  & \textbf{7.188} & \textbf{7.398} & \textbf{12900.36} & \textbf{5142671}
   & --- & TO & --- & ---
   & --- & TO & --- & --- \\
\rowcolor{lightgray}
17  & \textbf{16.212} & \textbf{16.562} & \textbf{12942.48} & \textbf{11023829}
   & --- & TO & --- & ---
   & --- & TO & --- & --- \\
\midrule
% ----------------------- GATES DATASET -----------------------
\multicolumn{13}{c}{$\blacktriangleright$
{\normalsize \gates{}}~\cite{tarzan2025} ::
[Query: $\exists \Diamond ( \mathit{Unlocker.Goal} )$]
$\blacktriangleleft$} \\
\midrule
\rowcolor{white}
3  & $\varepsilon$ & 0.013 & 7.79 & 26
   & ${\boldsymbol \varepsilon}$ & \textbf{0.006} & \textbf{5.99} & \textbf{18}
   & $\varepsilon$ & 0.054 & 18.86 & 18 \\
\rowcolor{lightgray}
5  & ${\boldsymbol \varepsilon}$ & \textbf{0.013} & \textbf{8.84} & \textbf{76}
   & 0.001 & 0.008 & 7.19 & 549
   & 0.001 & 0.055 & 19.01 & 549 \\
\rowcolor{white}
7  & ${\boldsymbol \varepsilon}$ & \textbf{0.014} & \textbf{11.23} & \textbf{151}
   & 0.110 & 0.122 & 21.08 & 32979
   & 0.035 & 0.092 & 22.79 & 32979 \\
\rowcolor{lightgray}
9  & \textbf{0.001} & \textbf{0.015} & \textbf{15.43} & \textbf{251}
   & 47.895 & 48.771 & 806.72 & 3071646
   & 5.228 & 6.509 & 451.71 & 3071646 \\
\rowcolor{white}
11  & \textbf{0.002} & \textbf{0.016} & \textbf{21.87} & \textbf{379}
   & --- & TO & --- & ---
   & --- & TO & --- & --- \\
\rowcolor{lightgray}
13  & \textbf{0.004} & \textbf{0.018} & \textbf{31.31} & \textbf{537}
   & --- & TO & --- & ---
   & --- & TO & --- & --- \\
\rowcolor{white}
15  & \textbf{0.006} & \textbf{0.020} & \textbf{44.01} & \textbf{708}
   & --- & TO & --- & ---
   & --- & TO & --- & --- \\
\rowcolor{lightgray}
17  & \textbf{0.009} & \textbf{0.023} & \textbf{60.85} & \textbf{922}
   & --- & TO & --- & ---
   & --- & TO & --- & --- \\
\midrule
% ----------------------- RING DATASET -----------------------
\multicolumn{13}{c}{$\blacktriangleright$
{\normalsize \ring{}}~\cite{tarzan2025} ::
[Query: $\exists \Diamond ( P_0.\mathit{Goal} \land P_1.\mathit{Goal} \land ... \land P_K.\mathit{Goal} )$]
$\blacktriangleleft$} \\
\midrule
\rowcolor{white}
2  & $\varepsilon$ & 0.013 & 7.84 & 59
   & ${\boldsymbol \varepsilon}$ &\textbf{0.006} & \textbf{6.14} & \textbf{45}
   & $\varepsilon$ & 0.054 & 18.83 & 45 \\
\rowcolor{lightgray}
4  & \textbf{0.001} & \textbf{0.015} & \textbf{12.40} & \textbf{542}
   & 0.020 & 0.029 & 11.56 & 7738
   & 0.010 & 0.065 & 19.52 & 7738 \\
\rowcolor{white}
6  & \textbf{0.011} & \textbf{0.025} & \textbf{48.96} & \textbf{3397}
   & 12.137 & 12.561 & 268.93 & 1180575
   & 3.406 & 3.715 & 128.87 & 1180575 \\
\rowcolor{lightgray}
8  & \textbf{0.204} & \textbf{0.225} & \textbf{687.77} & \textbf{47063}
   & --- & TO & --- & ---
   & --- & TO & --- & --- \\
\rowcolor{white}
10  & \textbf{0.272} & \textbf{0.295} & \textbf{897.00} & \textbf{52669}
   & --- & TO & --- & ---
   & --- & TO & --- & --- \\
\rowcolor{lightgray}
12  & \textbf{6.901} & \textbf{7.097} & \textbf{13049.36} & \textbf{1067623}
   & --- & TO & --- & ---
   & --- & TO & --- & --- \\
\rowcolor{white}
14  & --- & --- & OOM & ---
   & --- & TO & --- & ---
   & --- & TO & --- & --- \\
\rowcolor{lightgray}
16  & --- & --- & OOM & ---
   & --- & TO & --- & ---
   & --- & TO & --- & --- \\
\bottomrule
\end{tabular}
}
\end{table}
}
}
